# Supplementary material for: Probing nuclear effects with neutrino-induced charged-current neutral pion production
Source: arXiv:2002.05812 ancillary file (2024-08-24)
Supplement: Supplementary file 1 [file SupplementalMaterial1.pdf]

In Supplemental Material 1, we show the GiBUU (2019) predictions for the previous MINER $\nu$ A QE-like measurement of  $p_n$  and  $\delta\alpha_T$  [Phys. Rev. Lett.**121**, 022504 (2018)] in Fig. 1 below. This serves as a complementary comparison to those in the main article.

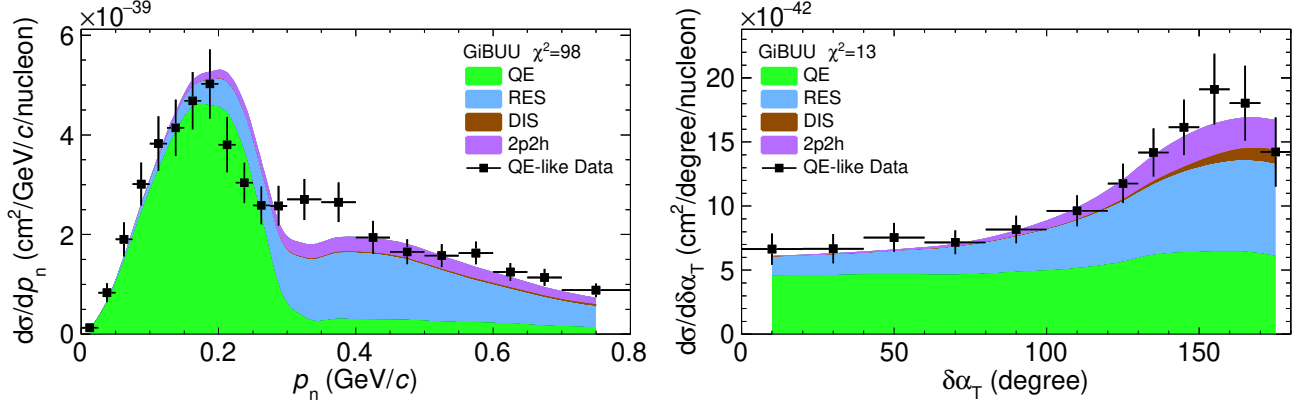

Figure 1: Cross sections in  $p_n$  and  $\delta\alpha_T$  from previous MINER $\nu$ A QE-like measurement [Phys. Rev. Lett.**121**, 022504 (2018)] compared to GiBUU (2019) predictions.

In addition, for all measured differential cross sections in the main article, the correlation matrices for the total uncertainty and the uncertainties from individual sources are presented. This is to help visualize the bin-by-bin correlation of the measured differential cross sections, and to accompany the numerical tables in Supplemental Material 2.

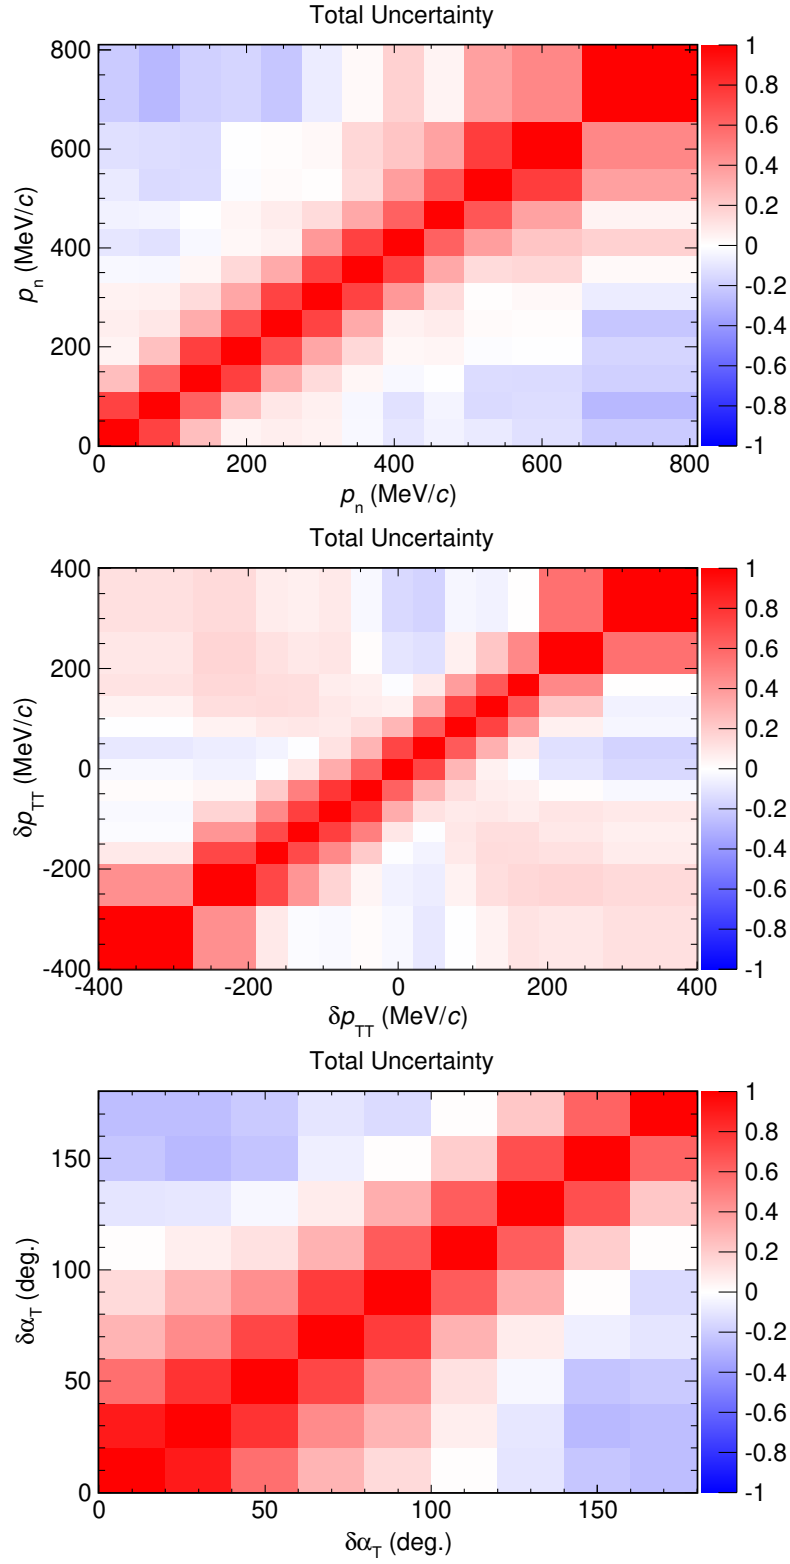

Figure 2: Total uncertainty correlation matrix for all variables.

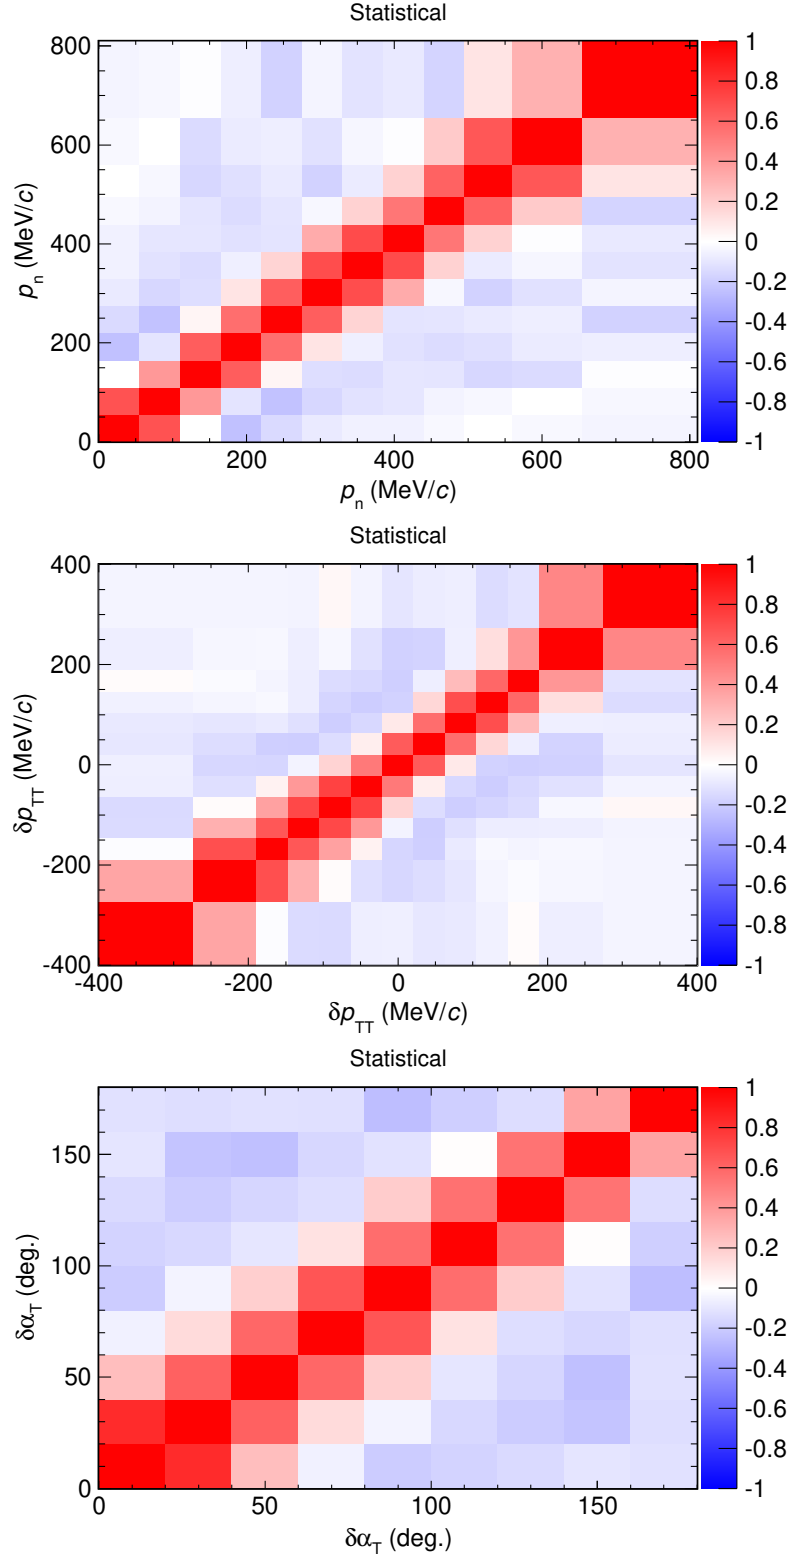

Figure 3: Statistical uncertainty correlation matrix for all variables.

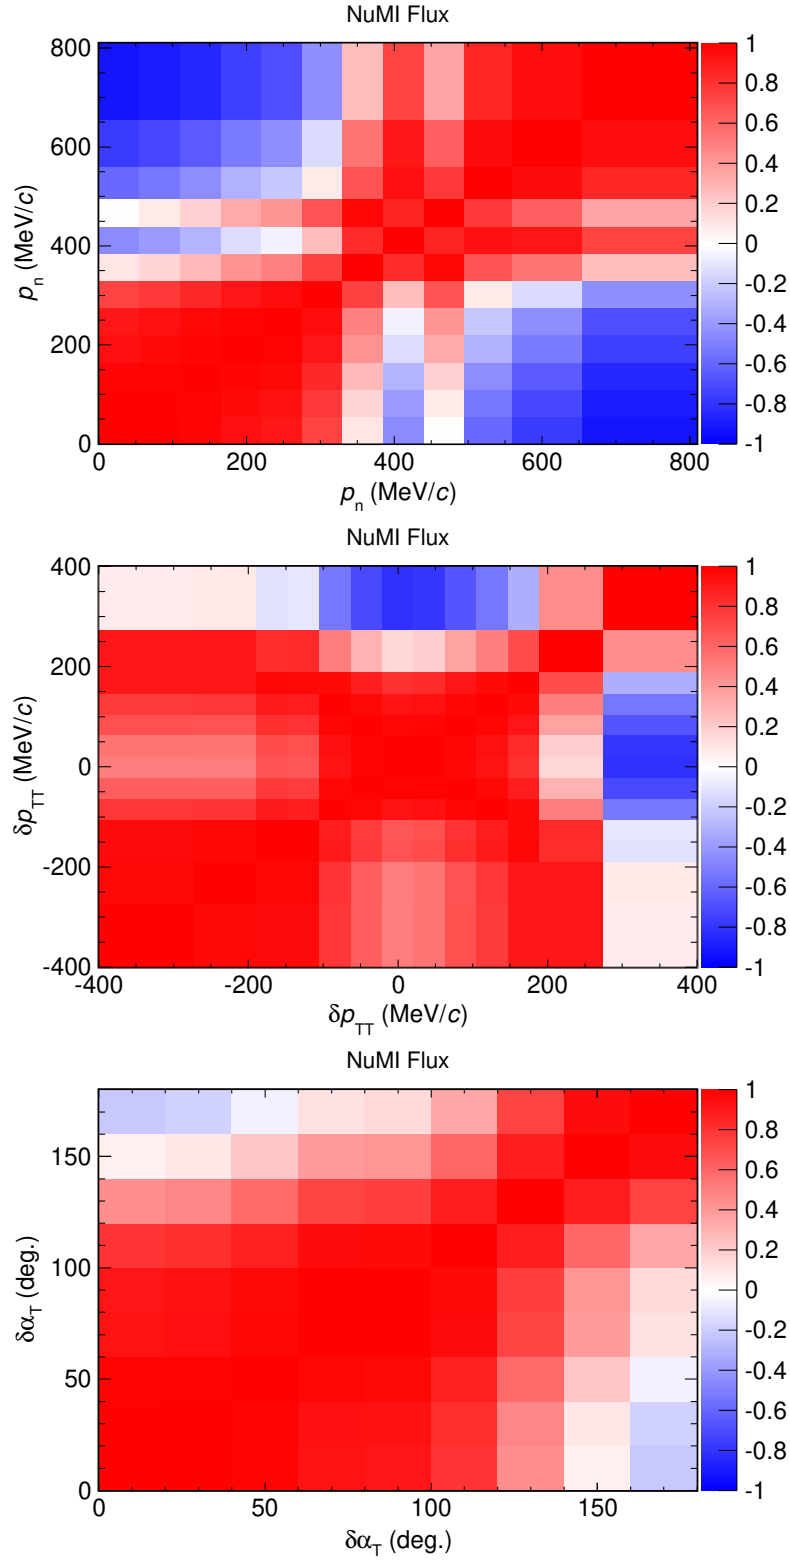

Figure 4: NuMI flux uncertainty correlation matrix for all variables.

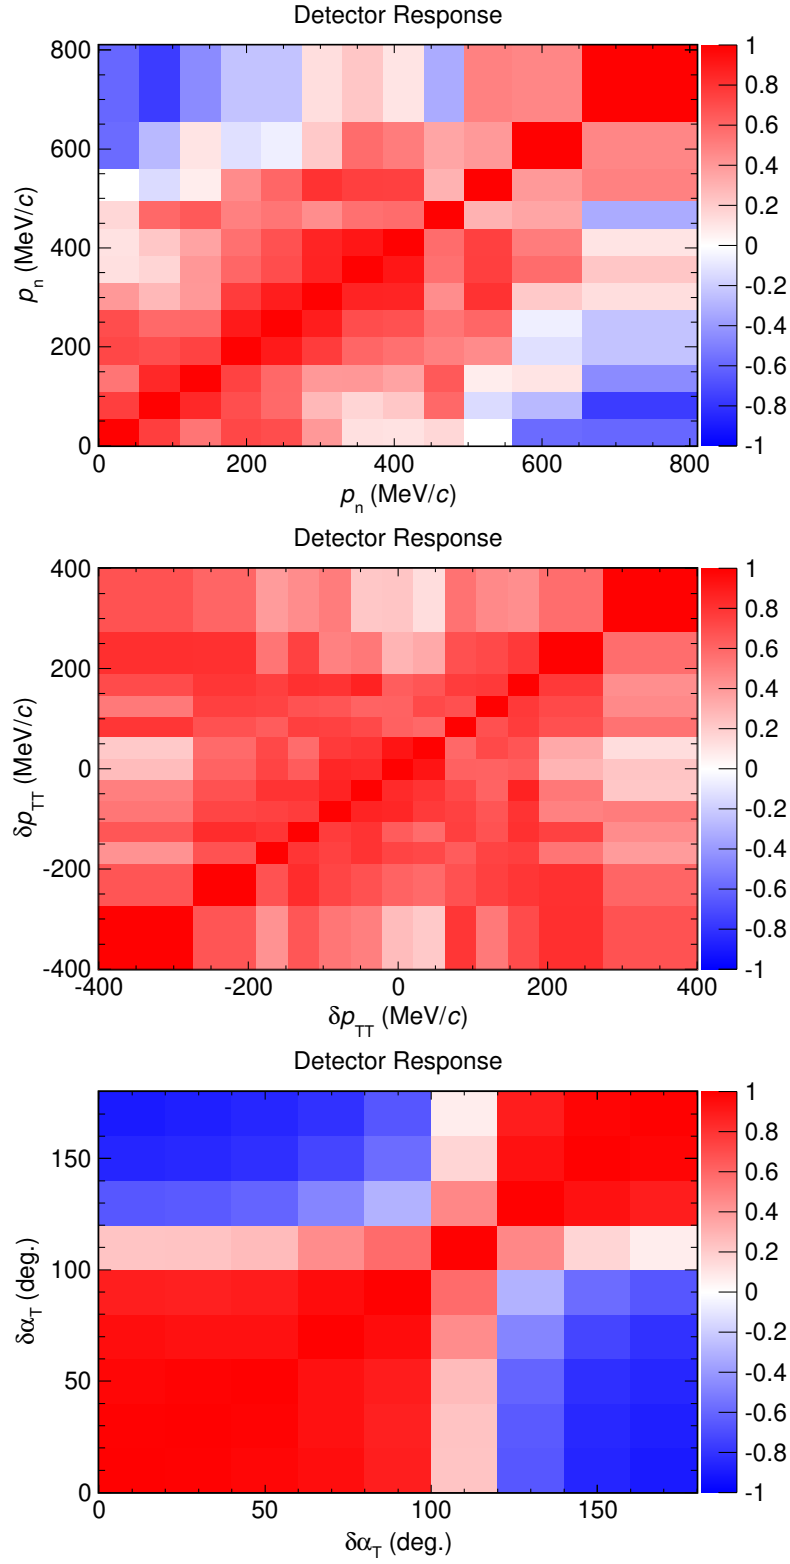

Figure 5: Detector response uncertainty correlation matrix for all variables.

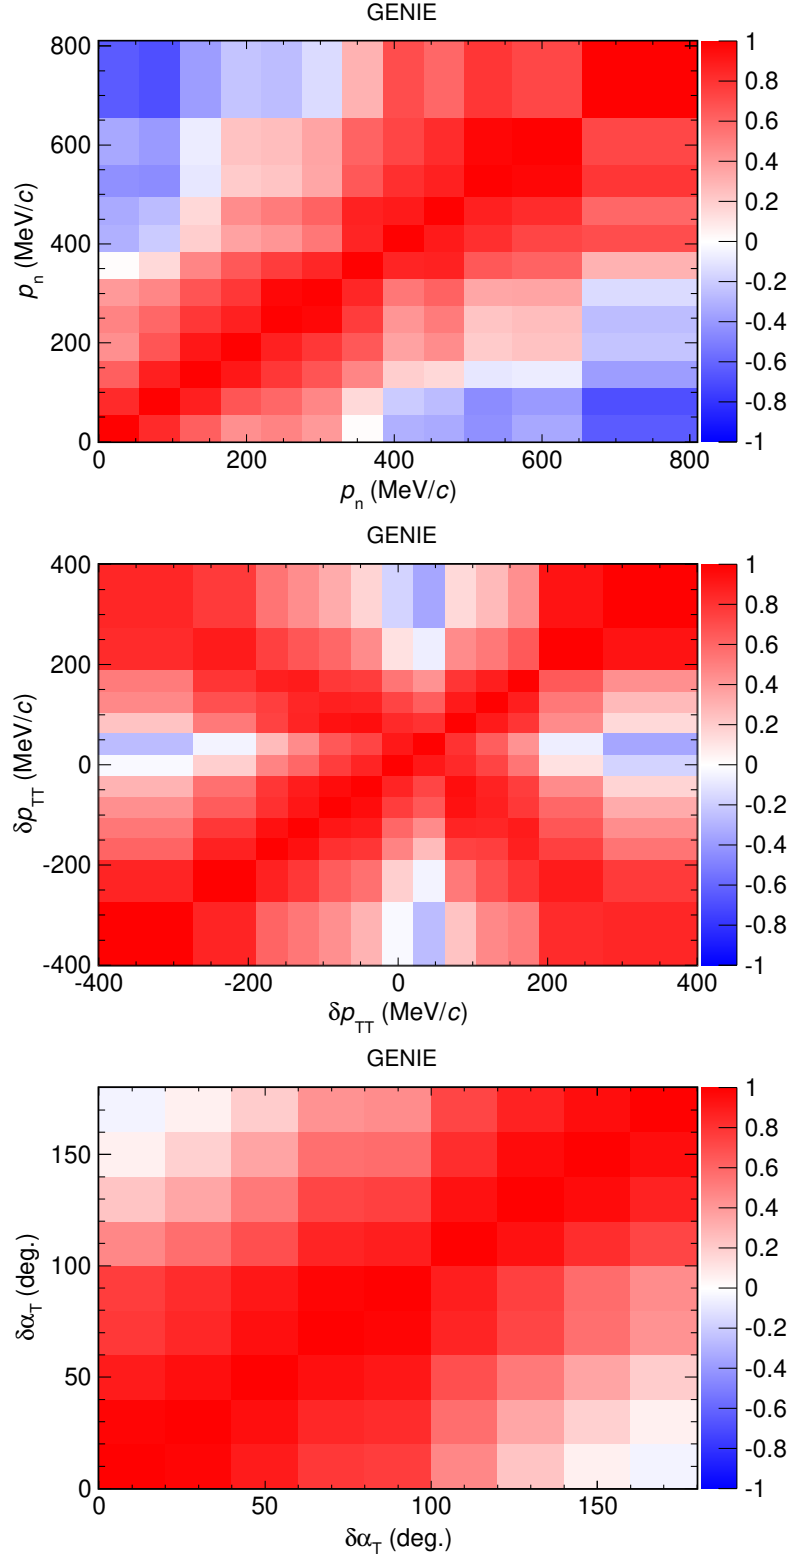

Figure 6: GENIE model uncertainty correlation matrix for all variables.
